# Supplementary material for: Spatiotemporal Event Graphs for Dynamic Scene Understanding
Source: arXiv:2312.07621 source file (2023-12-11)
Supplement: Supplementary file 1 [file appendixnumberbeamer.sty.tex]

\documentclass{article}
\usepackage{geometry}
\geometry{noheadfoot, margin=0.5in}
\usepackage{prerex}
\begin{document}
\thispagestyle{empty}
\begin{chart}
\end{chart}
\end{document}
